# Supplementary material for: Magnetic field estimation using Gaussian process regression for interactive wireless power system design
Source: arXiv:2510.19277 ancillary file (2025-10-22)
Supplement: Supplementary file 1 [file supplementary.pdf]

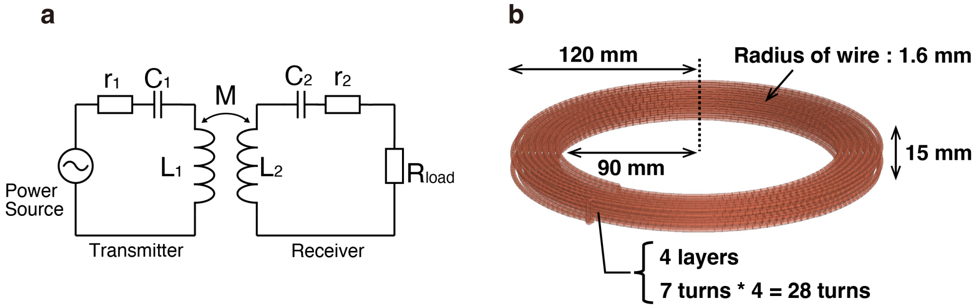


Supplementary Fig. 1: Configuration of coils and shields used in the study. **a** A circuit diagram for wireless power transmission. **b** The coil structure comprises 4 layers, each with an inner radius of 90 mm, an outer radius of 120 mm, and 7 turns, summing up to 28 turns with a height of 15 mm. Copper wire with a radius of 1.6 mm is used.

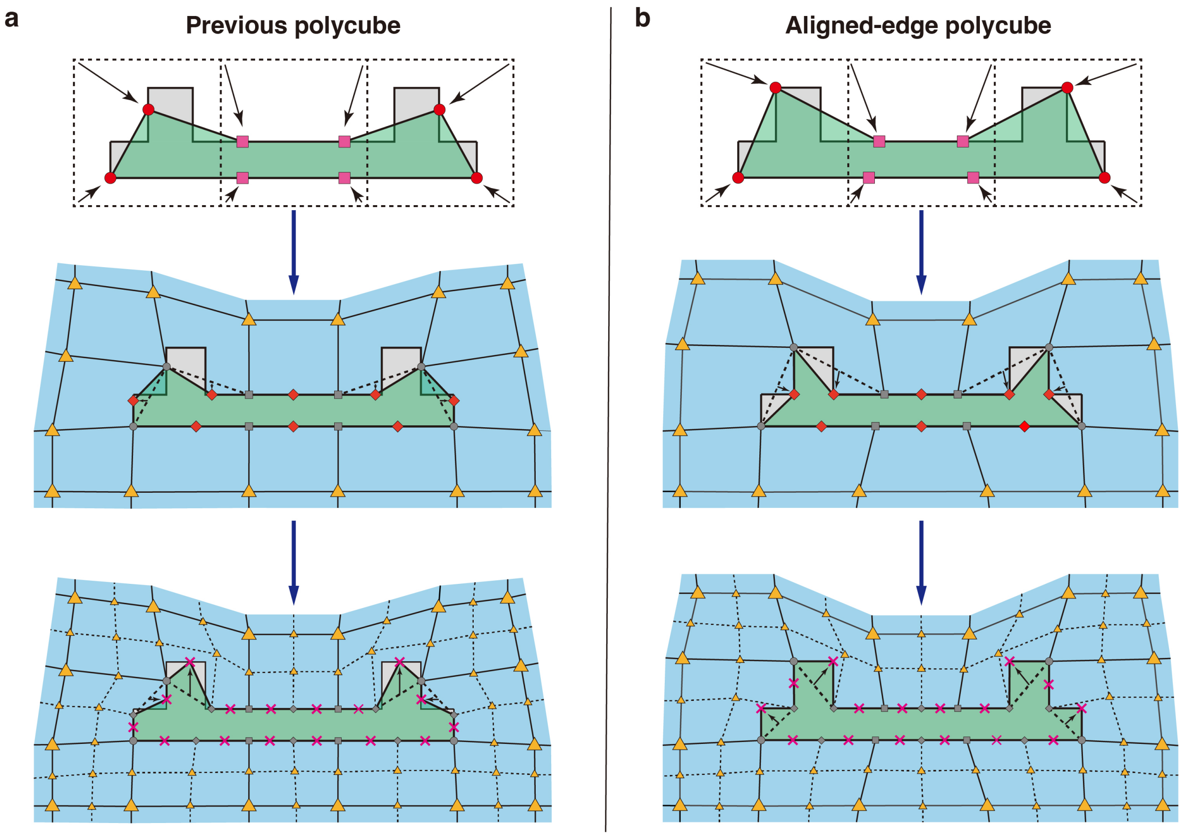


Supplementary Fig. 2: Conceptual comparison between previous polycube parameterization and proposed aligned-edge polycube mesh. **a** Previous polycube parameterization assumes smooth geometries, necessitating numerous points to accurately represent angular geometries like magnetic shields. **b** The aligned-edge polycube mesh reduces the number of required points by aligning them with the edges, offering a more efficient representation.

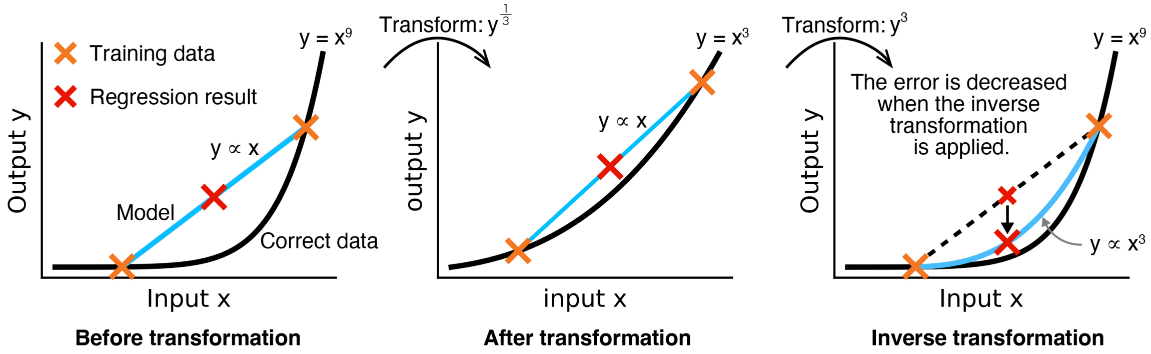


Supplementary Fig. 3: A simple example of improving accuracy through postprocessing linearization. When the correct model changes rapidly, it is difficult to represent it accurately with a small amount of training data. By performing the transformations described in the corresponding postprocessing section, our GPR model can be made more accurate. The error is decreased when the inverse transformation is applied.

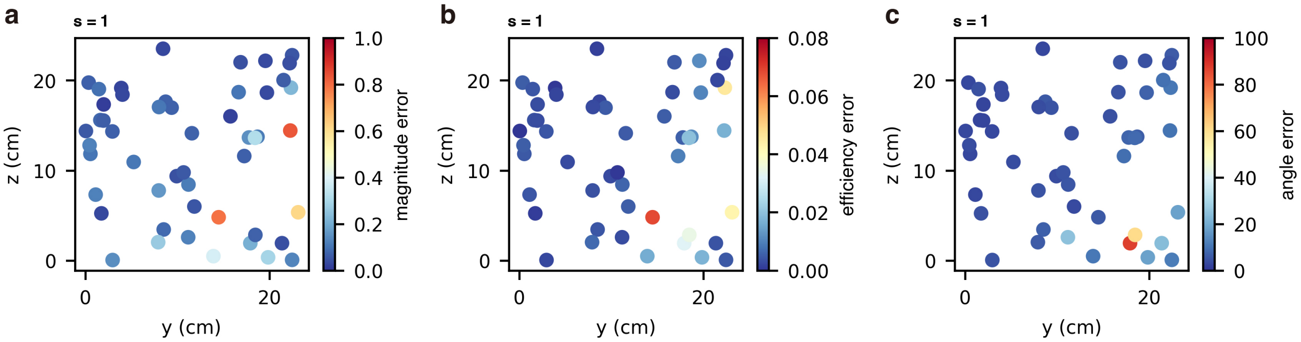


Supplementary Fig. 4: Estimation error maps. **a** Estimation error of the electromagnetic field magnitude when $s = 1$ (*i.e.*, without postprocessing). We note that one of the sample produces an error of approximately 90% before selecting an appropriate $s$ for postprocessing adjustment. **b** Estimation error of power transfer efficiency when $s = 1$. Similarly, we observe one of the sample produces an error of about 8% before the $s$ adjustment. **c** Estimation error of the electromagnetic field vector when $s = 1$. While many errors are below 10 degrees, some errors reach approximately 100 degrees and remain unchanged even with adjustments in $s$.

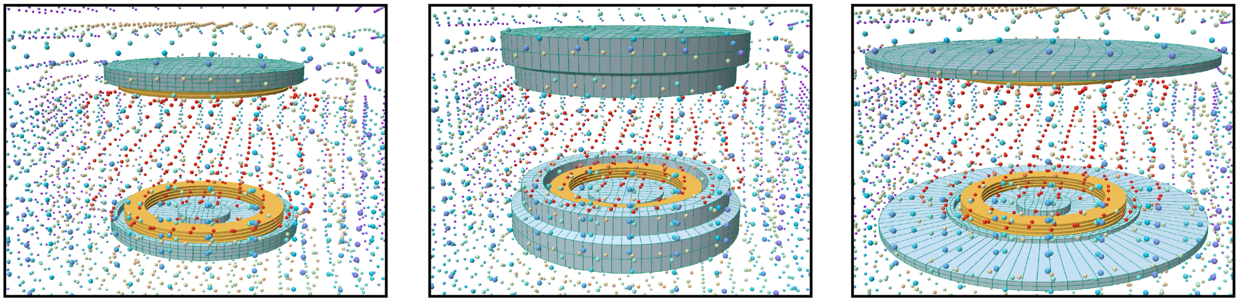

Supplementary Fig. 5: Example deformations of the shield. The proposed method has demonstrated robustness across various shield geometries, making it possible to predict behavior for diverse shapes.

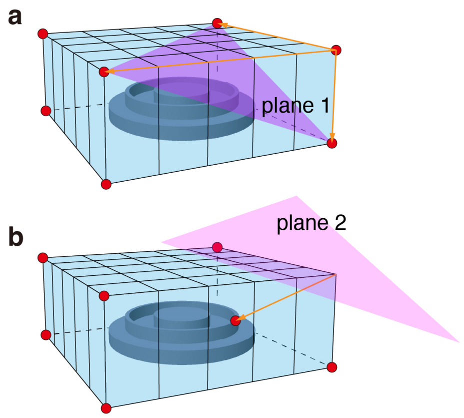


Supplementary Fig. 6: Corner point placement. **a** The plane passes through the adjacent corner points. **b** Points at the corners are moved to the nearest point from a plane that is parallel to the plane defined in Supplementary Fig. 6a, and that containing the point. **c** Shows the plane using the vector corresponding to moving the adjacent corner points. **d** Points at the edges are then moved to the nearest point from a plane parallel to the plane defined in Supplementary Fig. 6c and passing through the original point.

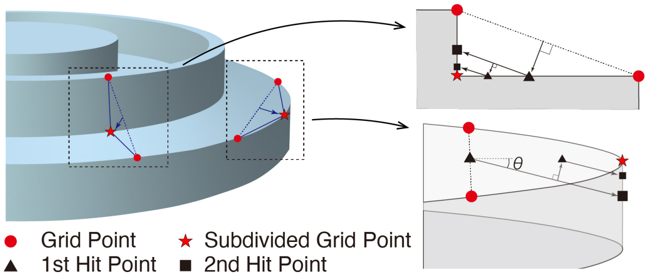


Supplementary Fig. 7: Approach to increment the subdivided grid points. First, we consider the path where two points are at a corner, and a sufficient gap exists between the straight line connecting them and the geometry of the object. In this case, we take the midpoint between those two points and move a point perpendicularly from there, designating this as our 1st hit point. Next, we find the intersection point of the line drawn from the moving point along the line connecting the original grid points and the object geometry, and we designate this as the 2nd hit point. We replace the initial two points with these new points and repeat the process until the points are sufficiently close to the edge. This determines the next grid point. Next, we consider the path where two points are also at a corner, but there is an insufficient gap between the straight line connecting them and the geometry of the object. Intuitively, one would aim to position the points outside the disk-shaped part in the corner. In our case, we take the midpoint as the 1st hit point and define the point where a line at an angle $\theta$ (a set value) from the 1st hit point intersects with the surface of the geometry, as our 2nd hit point. By iterating this process, the next grid point can be determined.

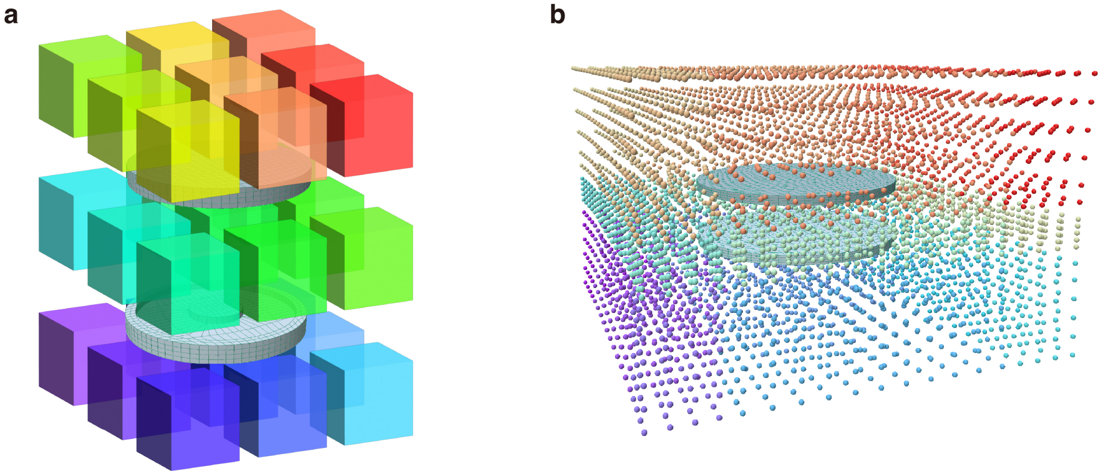


Supplementary Fig. 8: The 27 blocks used for selecting the six points of interest in active learning. The 27 blocks are divided into three areas: between the shields or outside of them. Each area is divided into a $3 \times 3$ grid, resulting in 9 blocks each. **a** Schematic diagram. **b** Actual division of the estimation points.

Supplementary Table 1: Comparison between methods for magnetic field computation.

| | MoM | Knaisch's method [1] | Our method |
|---|---|---|---|
| Calculation speed[1] | × | ✓ | ✓ |
| Data collection efficiency[2] | × | × | ✓ |
| Estimation Accuracy[3] | ✓ | × | ✓ |
| Geometry freedom[4] | ✓ | × | ✓ |
| Estimation range[5] | ✓ | × | ✓ |
| Interactivity[6] | × | × | ✓ |

[1] Typical per-query runtimes: MoM $\approx$ 1758 s; Knaisch's method $\approx$ 1 s; our estimator $\approx$ 130 ms.

[2] Our active learning method calculates the distance within the model, allowing us to select more necessary data points for the model. Prior approaches use the linear distance between data points, which do not correspond to the distance within the model.

[3] Representative errors: our method $\approx$ 6%, aided by an adaptive exterior grid that accounts for shield geometry; Knaisch's method $\approx$ 20%, as it does not account for the geometric relationship of sampled points to the shield.

[4] Geometric flexibility: our 3D modeling supports broader geometry variations, whereas Knaisch's method is more restricted.

[5] Estimation domain: our method predicts fields throughout an 80 cm cubic volume around the system; Knaisch's method estimates only a small number of probe points.

[6] Our method enables interactive estimation in under 130 ms. Knaisch's approach focuses on model optimization and does not address interactivity.

Supplementary Table 2: Comparison of methods for expressing shield geometries

| | Fixed[1] | Compact[2] | Linear[3] |
|---|---|---|---|
| **our method** | ✓ | ✓ | ✓ |
| Multi-view projection [2] | ✓ | × | × |
| Voxel [3, 4] | ✓ | × | × |
| SDF on a Cartesian grid [5] | ✓ | × | ✓ |
| Point cloud [6] | × | ✓ | × |
| Triangle mesh [7] | × | ✓ | ✓ |
| B-Rep [8] | × | ✓ | ✓ |

[1] Fixed: Input and output vectors with fixed length facilitate accurate regression.
[2] Compact: The dimension of the input and output vectors should be as small as possible to avoid redundancy.
[3] Linear: The relationship between input and output should be as linear as possible to avoid complicated models, which are difficult to train from a small amount of data points.

Supplementary Table 3: Comparison of methods for selecting evaluation grid points

| | Fixed[1] | Compact[2] | Linear[3] |
|---|---|---|---|
| **our method** | ✓ | ✓ | ✓ |
| Voxel grid [3, 4] | ✓ | ✓ | × |
| Values on a Cartesian grid [9] | ✓ | ✓ | × |
| Tetrahedra mesh [10] | × | ✓ | ✓ |

[1] Fixed: Input and output vectors with fixed-length facilitate accurate regression.

[2] Compact: The dimension of the input and output vectors should be as small as possible to avoid redundancy.

[3] Linear: The relationship between input and output should be as linear as possible to avoid complicated models, which are difficult to train from a small amount of data points.

Supplementary Table 4: Estimation's relative error improvement with our proposed method

| Method | | Error rate |
|---|---|---|
| Grid | fixed grid | 122.3% |
| | proposed grid | 94.1% |
| | proposed grid and optimized GPR | 15.1% |
| Active learning | before (average error at 6 points) | 162.8% |
| | after (average error at 6 points) | 54.5% |
| Transformation | $k = 1$ | 14.1% |
| | $k = 20$ | 5.5% |

Supplementary Table 5: The shield geometry and the position parameters.

| Shield geometry · Position | min | max | interval |
|---|---|---|---|
| $r_1$ (mm) | 140 | 200 | 20 |
| $r_2$ (mm) | 130 | 190 | 20 |
| $r_3$ (mm) | 40 | 70 | 30 |
| $d$ (mm) | 10 | 70 | 20 |
| $h_1$ (mm) | 10 | 30 | 10 |
| $h_2$ (mm) | 0 | 30 | 10 |
| The reference position (cm) | 5 | - | - |
| $y$ (cm) | 0 | 24 | 2 |
| $z$ (cm) | 0 | 24 | 2 |

# References


1. Knaisch, K. & Gratzfeld, P. Gaussian process surrogate model for the design of circular, planar coils used in inductive power transfer for electric vehicles. *IET Power Electronics* **9,** 2786–2794 (2016).
2. Su, H., Maji, S., Kalogerakis, E. & Learned-Miller, E. Multi-view Convolutional Neural Networks for 3D Shape Recognition. *2015 IEEE International Conference on Computer Vision (ICCV),* 945–953 (2015).
3. Wu, Z. *et al.* 3D ShapeNets: A Deep Representation for Volumetric Shapes. *Proceedings of the IEEE conference on computer vision and pattern recognition,* 1912–1920 (2015).
4. Wang, P. S., Liu, Y., Guo, Y. X., Sun, C. Y. & Tong, X. O-CNN: octree-based convolutional neural networks for 3D shape analysis. *ACM Trans. Graph.* **36,** 72:1–72:11 (2017).
5. Calakli, F. & Taubin, G. SSD: Smooth Signed Distance Surface Reconstruction. *Computer Graphics Forum* **30,** 1993–2002 (2011).
6. Qi, C. R., Su, H., Mo, K. & Guibas, L. J. PointNet: Deep Learning on Point Sets for 3D Classification and Segmentation. *Proceedings of the IEEE conference on computer vision and pattern recognition,* 652–660 (2017).
7. Schroeder, W. J., Zarge, J. A. & Lorensen, W. E. Decimation of triangle meshes. *Proceedings of the 19th annual conference on Computer graphics and interactive techniques,* 65–70 (1992).
8. Zhu, H. & Menq, C. H. B-Rep model simplification by automatic fillet/round suppressing for efficient automatic feature recognition. *Computer-Aided Design* **34,** 109–123 (2002).
9. Chen, S., Xu, K. & Li, Z. Cartesian grid method for gas kinetic scheme on irregular geometries. *Journal of Computational Physics* **326,** 862–877 (2016).
10. Weatherill, N. P. & Hassan, O. Efficient three-dimensional Delaunay triangulation with automatic point creation and imposed boundary constraints. *International Journal for Numerical Methods in Engineering* **37,** 2005–2039 (1994).
